# Supplementary material for: The Shape of Alerts: Detecting Malware Using Distributed Detectors by Robustly Amplifying Transient Correlations
Source: arXiv:1803.00883 source file (2018-03-01)
Supplement: Supplementary file 1 [file overhead-appendix.tex]

\textbf{Local detectors.} Generating a single FV, which is a 1-sec
histogram of system calls, on a local host is equivalent to performing
2,500 (system call frequency) direct table lookups on average and
incrementing corresponding counters. Projection on a PCA basis
requires computing 10 dot products. Finally, running an LD, which is
Random Forest in our case, results in performing 330 scalar
comparisons on average. At 1 second per FV, the overheads of such an
LD are negligible.
%Finally, if an FV is suspicious, a node projects it on the ten dimensional basis, which is equivalent to ten dot products.

\textbf{Data transfer.} Each FV is composed of 10 floating point
numbers (40 bytes total if assuming single precision format). In the
phishing experiment 1086 hosts transfer (in aggregate) $\sim 40
KB/sec$; data transfer rate in waterhole setting is a little bit
higher: $\sim 4,450$ hosts transfer (in aggregate) $\sim 174 KB/sec$.
In both cases we assume Shape GD using pure time-based filtering with
1 hour and 6 sec neighborhood time windows respectively.

If Shape GD employs structural filtering on top of the time-based one,
then data transfer depends on the number of emails floating in a
network or on the number of servers. In both cases, data transfer
scales linearly with the number of emails and servers. When applying
the most fine-grained structural filtering in our experiments, the
nodes susceptible to phishing attacks transfer $\sim 4 KB/sec$ per
email and the nodes susceptible to waterhole attacks send $\sim 40
KB/sec$ per server when using 1 hour and 25 sec neighborhood windows
respectively.

\textbf{Server computations.} After receiving a batch of alert-FVs,
Shape GD performs lightweight computations.
%: it performs mostly additive operations and few multiplicative
%operations when computing one dot product. Binning %(estimating pmf
%of incoming FVs)
Overhead of binning scales linearly with the number of alert-FVs in a
batch; each binning operation is a direct table lookup together with
counter increment. Calculating ShapeScore, which is Wasserstein
distance, results in a sequence of addition operations, whose total
number is equal to the dimensionality of FVs, which is 10, multiplied
by the number of bins, which is 50. To summarize, Shape GD's computational
requirements are fairly light-weight.
